# Supplementary material for: DARN: Dynamic Adaptive Regularization Networks for Efficient and Robust Foundation Model Adaptation
Source: arXiv:2511.04766 source file (2025-11-06)
Supplement: Supplementary file 1 [file X_suppl.tex]

\clearpage
\setcounter{page}{1}
\maketitlesupplementary

\appendix
\section{Additional Ablations}
Complexity loss weight $\beta$ sweep indicates $\beta=0.05$ provides the best trade-off in shorter runs.

\section{Hyperparameter Sensitivity}
Learning rate sweep for full fine-tuning shows \num{1e-4} with warmup performed best in our setup.

\section{Computational Details}
Hardware: NVIDIA H100 80GB. Inference throughput/latency measured with CUDA events, FP16.

\section{Robustness Evaluation Details}
Scope: Frozen backbone. FGSM with $\epsilon=8/255$ (single-step). Common Corruptions per standard protocol; mean mCE averaged across types and severities.
